# Supplementary material for: Graph Learning Across Data Silos
Source: arXiv:2301.06662 source file (2025-02-17)
Supplement: Supplementary file 1 [file supplementary.tex]

\justifying

In the supplementary material, we explain how MRMTL and Ditto are applied to jointly learn local graphs and the consensus graph.

\vspace{1.5em}
\noindent\textbf{Application of MRMTL}
\vspace{0.8em}

As described in \cite{liu2022privacy}, MRMTL is a privacy-preserving algorithm that further considers data heterogeneity to learn models in  cross-silo federated learning. Applying this algorithm to multiple graph learning is equivalent to solving the following problem
\begin{align}
   &\underset{\mathbf{w}_1,\dots, \mathbf{w}_I\in \mathcal{W}}{\min}  \sum_{i=1}^I l_i(\mathbf{w}_i) \notag\\
   = &\underset{\mathbf{w}_1,\dots, \mathbf{w}_I\in \mathcal{W}}{\min} \sum_{i=1}^I \underbrace{\frac{1}{N_i}  \mathbf{z}_{i}^{\top}\mathbf{w}_i - \alpha\mathbf{1}^{\top} \log\left(\mathbf{S}\mathbf{w}_i\right) + 2\beta\lVert \mathbf{w}_i\rVert_2^2}_{{g}_i(\mathbf{w}_i)}  \notag\\
   &\;\;\;\;\;\;\;\;\;\;\;\;\;\;\;\;+ \frac{\varsigma}{2} \lVert \mathbf{w}_i - \mathbf{w}_{\mathrm{avg}} \rVert_2^2, \label{R1}   
\end{align}
where $\varsigma$ is the weight before the regularizer. In the above model, $\mathbf{w}_{\mathrm{avg}} = \frac{1}{I} \sum_{i=1}^I \mathbf{w}_i$ is called the ``average graph", which corresponds to the consensus graph in our model.

Then, following the MRMTL algorithm, problem \eqref{R1} is solved via Algorithm A1.

\begin{algorithm}[htbp] 
\caption{MRMTL for solving \eqref{R1}} 
\begin{algorithmic}[1] %这个1 表示每一行都显示数字
\REQUIRE  %算法的输入参数：Input
$\alpha$, $\beta$,  $\varsigma$, and  signals $\mathbf{X}_1$,$\dots$, $\mathbf{X}_I$ \\
\STATE  \textbf{Initialize} $ \mathbf{w}_{i}^{(0)}$ and $\mathbf{w}_{\mathrm{avg}}^{(0)}$ for $i =1,\dots,I$. \\
\FOR{$t = 1,\dots, T$}
\STATE {\color{red}\emph{/\,/\,\,Update $\mathbf{w}_1,\dots,\mathbf{w}_I$ in parallel in  local clients}} 
\FOR{$i = 1,\dots, I$ in parallel}
\STATE Receive $\mathbf{w}_{\mathrm{avg}}^{(t-1)}$ from the central server

\STATE Let $\mathbf{w}_{i}^{(t)} = \mathbf{w}_{i}^{(t-1)}$ 

\STATE Update $\mathbf{w}_{i}^{(t)} = \mathbf{w}_{i}^{(t)} - \eta  \nabla_{\mathbf{w}_{i}} l_i( \mathbf{w}_{i}^{(t)})$ $K$ times, where $\nabla_{\mathbf{w}_{i}} l_i( \mathbf{w}_{i}^{(t)}) = \nabla_{\mathbf{w}_{i}} g_i(\mathbf{w}_{i}^{(t)}) + \varsigma (\mathbf{w}_{i}^{(t)} - \mathbf{w}_{\mathrm{avg}}^{(t-1)})$ 

\STATE Send $\mathbf{\Delta}_{i}^{(t)} = \mathbf{w}_{i}^{(t)} - \mathbf{w}_{i}^{(t-1)}$ back to the central server
\ENDFOR

\STATE {\color{red}\emph{/\,/\,\,Update $\mathbf{w}_{\mathrm{avg}}$ in the central server}} 
\STATE The central server updates $\mathbf{w}_{\mathrm{avg}}^{(t)} = \mathbf{w}_{\mathrm{avg}}^{(t-1)} + \frac{1}{I} \sum_{i}^{I} \mathbf{\Delta}_{i}^{(t)} $

\ENDFOR
\RETURN $\mathbf{w}_1^{(T)}$, \ldots ,$\mathbf{w}_I^{(T)}$ %算法的返回值
\end{algorithmic}
\label{A1}
\end{algorithm}

\vspace{1.5em}
\noindent\textbf{Application of Ditto }
\vspace{0.8em}

The second algorithm Ditto \cite{li2021ditto} is another privacy-preserving algorithm in personalized federated learning, which considers statistically heterogeneous data. Applied to the problem of multiple graph learning, the Ditto objective function of each local client is as follows.
\begin{align}
   &\underset{\mathbf{w}_i\in \mathcal{W} }{\min}   l_i(\mathbf{w}_i) \notag\\
   = &\underset{\mathbf{w}_i\in \mathcal{W} }{\min} \underbrace{\frac{1}{N_i}  \mathbf{z}_{i}^{\top}\mathbf{w}_i - \alpha\mathbf{1}^{\top} \log\left(\mathbf{S}\mathbf{w}_i\right) + 2\beta\lVert \mathbf{w}_i\rVert_2^2}_{{g}_i(\mathbf{w}_i)} \notag\\
   &\;\;\;\;\;\;\;\;\;+ \frac{\varsigma}{2} \lVert \mathbf{w}_i - \mathbf{w}_{\mathrm{avg}} \rVert_2^2\notag\\
   & \mathrm{s.t.}\; \mathbf{w}_{\mathrm{avg}} \in \underset{\mathbf{w}\in \mathcal{W} }{ \mathrm{arg}\min} \sum_{i}^{I} \frac{N_i}{N_{all}} g_i(\mathbf{w}).
   \label{R2}   
\end{align}

In problem \eqref{R2}, the ``average graph" $\mathbf{w}_{\mathrm{avg}}$ belongs to the results of the celebrated FedAvg formulation \cite{mcmahan2017communication}, where the objective function is the weighted sum of all local loss. Then, following the Ditto algorithm, problem \eqref{R2} is solved via Algorithm A2.

\begin{algorithm}[htbp] 
\caption{Ditto for solving \eqref{R2}} 
\begin{algorithmic}[1] %这个1 表示每一行都显示数字
\REQUIRE  %算法的输入参数：Input
$\alpha$, $\beta$,  $\varsigma$, and  signals $\mathbf{X}_1,\dots,\mathbf{X}_I$ \\
\STATE  \textbf{Initialize} $ \mathbf{w}_{i}^{(0)}$  and $\mathbf{w}_{\mathrm{avg}}^{(0)} $ for $i =1,\dots,I$.\\
\FOR{$t = 0,\dots, T-1$}
\STATE {\color{red}\emph{/\,/\,\,Update $\mathbf{w}_1,\dots,\mathbf{w}_I$ in parallel in  local clients}} 
\FOR{$i = 1,\dots, I$ in parallel}
\STATE Receive $\mathbf{w}_{\mathrm{avg}}^{(t)}$ from the central server

\STATE Let  $\mathbf{v}_{i}^{(t)} = \mathbf{w}_{\mathrm{avg}}^{(t)}$

\STATE Update   $\mathbf{v}_{i}^{(t)} = \mathbf{v}_{i}^{(t)}  -\eta_1  \nabla_{\mathbf{v}_{i}} g_i(\mathbf{v}_{i}^{(t)})$  $K$ times

\STATE Update   $\mathbf{w}_{i}^{(t)} = \mathbf{w}_{i}^{(t)}  -\eta_2  \nabla_{\mathbf{w}_{i}} \left( g_i(\mathbf{w}_{i}^{(t)}) + \varsigma(\mathbf{w}_{i}^{(t)} - \mathbf{w}_{\mathrm{avg}}^{(t)}) \right)$ 

\STATE Send $\mathbf{\Delta}_{i}^{(t)} = \mathbf{v}_{i}^{(t)} - \mathbf{w}_{\mathrm{avg}}^{(t)}$ back to the central server
\ENDFOR

\STATE {\color{red}\emph{/\,/\,\,Update $\mathbf{w}_{\mathrm{avg}}$ in the central server}} 
\STATE The central server update $\mathbf{w}_{\mathrm{avg}}^{(t+1)} = \mathbf{w}_{\mathrm{avg}}^{(t)} + \sum_{i}^{I} \frac{N_i}{N_{all}} \mathbf{\Delta}_{i}^{(t)} $

\ENDFOR
\RETURN $\mathbf{w}_1^{(T)}$, \ldots ,$\mathbf{w}_I^{(T)}$ %算法的返回值
\end{algorithmic}
\label{A2}
\end{algorithm}
